# Supplementary material for: 3D Multi-Object Tracking Using Graph Neural Networks with Cross-Edge Modality Attention
Source: arXiv:2203.10926 source file (2022-05-14)
Supplement: Supplementary file 1 [file depr_appendix.tex]

%%%%%%%%%% Merge with supplemental materials %%%%%%%%%%
\clearpage

\setlength{\belowcaptionskip}{0pt}

\begin{strip}
\begin{center}
\vspace{-5ex}
\textbf{\LARGE \bf
3D Multi-Object Tracking Using Graph Neural Networks with\\\vspace{0.5ex}Cross-Edge Modality Attention} \\
\vspace{3ex}

\Large{\bf- Supplementary Material -}\\
\vspace{0.4cm}
\normalsize{Martin B\"uchner and Abhinav Valada}
\end{center}
\end{strip}

%%%%%%%%%% Merge with supplemental materials %%%%%%%%%%
\setcounter{section}{0}
\setcounter{equation}{0}
\setcounter{figure}{0}
\setcounter{table}{0}
\setcounter{page}{1}
\makeatletter

%%%%%%%%%% Prefix a "S" to all equations, figures, tables and reset the counter %%%%%%%%%%

\footnote{Department of Computer Science, University of Freiburg, Germany.\\
}%

\normalsize

In this supplementary material, we (i) provide more details about the dataset and the challenges that we are organizing based on the Panoptic nuScenes benchmark that we introduce in this work, (ii) present class-wise panoptic segmentation results, and (iii) extend the correlation analysis between semantic segmentation, object detection, multi-object tracking, and panoptic tracking.

\section{Additional Dataset Details}
This section presents further details about the Panoptic nuScenes dataset and annotations.

\noindent\textit{Dynamic and Diverse Scenes}: Panoptic nuScenes was primarily collected in dense urban environments with many dynamic agents. Such scenes include those near intersections and construction sites, which are of high traffic density and have the potential for interesting driving situations (e.g. jaywalkers, lane changes, turning). The scenes are also diverse in terms of, among others, geographical location (i.e. left-hand versus right-hand drive), weather, and lighting conditions. \figref{fig:annnotation_example} shows example panoptic segmentation annotations overlaid on the camera image.

\begin{figure}
\centering
\includegraphics[width=1.0\linewidth]{./images/panoptic_annotation_examples.pdf}
\caption{Front camera view of panoptic annotation examples, including construction zones (row 1), junctions (row 2), nighttime (row 3 left) and bendy bus (row 3 right). 
We can see that the annotations accurately outline vehicle wheels, rather than including nearby ground points (row 4).}
\label{fig:annnotation_example}
\end{figure}

\begin{figure*}
\centering
\footnotesize
{% for the vertical padding
\begin{tabular}{P{0.4cm}P{5.5cm}P{5.5cm}P{5.5cm}}
\multicolumn{4}{c}{Semantic Segmentation} \\
&\raisebox{-0.4\height}{\includegraphics[width=\linewidth,frame]{images/semantic0029-0020.jpg}} & \raisebox{-0.4\height}{\includegraphics[width=\linewidth,frame]{images/semantic0030-0014.jpg}} & \raisebox{-0.4\height}{\includegraphics[width=\linewidth,frame]{images/semantic0031-0018.jpg}} \\
&\raisebox{-0.4\height}{(a)} & \raisebox{-0.4\height}{(b)} &  \raisebox{-0.4\height}{(c)} \\
\\
&\raisebox{-0.4\height}{\includegraphics[width=\linewidth,frame]{images/semantic0035-0002.jpg}} & \raisebox{-0.4\height}{\includegraphics[width=\linewidth,frame]{images/semantic0036-0000.jpg}} & \raisebox{-0.4\height}{\includegraphics[width=\linewidth,frame]{images/semantic0039-0000.jpg}} \\
&\raisebox{-0.4\height}{(d)} & \raisebox{-0.4\height}{(e)} &  \raisebox{-0.4\height}{(f)} \\
\\\midrule
\multicolumn{4}{c}{Panoptic Segmentation} \\
&\raisebox{-0.4\height}{\includegraphics[width=\linewidth,frame]{images/panoptic0011-0018.jpg}} & \raisebox{-0.4\height}{\includegraphics[width=\linewidth,frame]{images/panoptic0017-0010.jpg}} & \raisebox{-0.4\height}{\includegraphics[width=\linewidth,frame]{images/panoptic0018-0001.jpg}} \\
&\raisebox{-0.4\height}{(g)} & \raisebox{-0.4\height}{(h)} &  \raisebox{-0.4\height}{(i)} \\
\\
&\raisebox{-0.4\height}{\includegraphics[width=\linewidth,frame]{images/panoptic0002-0006.jpg}} & \raisebox{-0.4\height}{\includegraphics[width=\linewidth,frame]{images/panoptic0026-0003.jpg}} & \raisebox{-0.4\height}{\includegraphics[width=\linewidth,frame]{images/panoptic0045-0000.jpg}} \\
&\raisebox{-0.4\height}{(j)} & \raisebox{-0.4\height}{(k)} &  \raisebox{-0.4\height}{(l)} \\
\\\midrule
\multicolumn{4}{c}{Panoptic Tracking} \\
{\rotatebox[origin=c]{90}{(m)}}
&\raisebox{-0.4\height}{\includegraphics[width=\linewidth,frame]{images/panoptic0000.jpg}} & \raisebox{-0.4\height}{\includegraphics[width=\linewidth,frame]{images/panoptic0001.jpg}} & \raisebox{-0.4\height}{\includegraphics[width=\linewidth,frame]{images/panoptic0002.jpg}} \\
&\raisebox{-0.4\height}{t-2} & \raisebox{-0.4\height}{t-1} &  \raisebox{-0.4\height}{t} \\
\\
{\rotatebox[origin=c]{90}{(n)}}
&\raisebox{-0.4\height}{\includegraphics[width=\linewidth,frame]{images/panoptic0023.jpg}} & \raisebox{-0.4\height}{\includegraphics[width=\linewidth,frame]{images/panoptic0024.jpg}} & \raisebox{-0.4\height}{\includegraphics[width=\linewidth,frame]{images/panoptic0025.jpg}} \\
&\raisebox{-0.4\height}{t-2} & \raisebox{-0.4\height}{t-1} &  \raisebox{-0.4\height}{t} \\
\end{tabular}}
\caption{Example annotations from our Panoptic nuScenes dataset. Figures~(a)-(f) show semantic segmentation annotations, Figures~(g)-(h) show panoptic segmentation annotations, and Figures~(m) and (n) show panoptic tracking annotations.}
\label{fig:visual_ablation}
\end{figure*}

\noindent\textit{Instance Statistics}: We present additional analysis of object instances that are present in the Panoptic nuScenes dataset, both from a scan-wise and sequence-wise perspective. \figref{fig:instances_scan_wise} shows the distribution of non-moving and moving scan-wise instances for various semantic classes. For common classes such as \emph{adult} and \emph{car}, we have 152k and 114k moving scan-wise instances. For rarer classes such as police and construction vehicles, there are 882 and 298 moving scan-wise instances, which is a non-trivial amount.

\begin{figure}
\centering
\includegraphics[width=\linewidth]{./images/instances_scan_wise.pdf}
\caption{Number of scan-wise instances, sorted by the number of moving instances. Note that the y-axis is in log scale.}
\label{fig:instances_scan_wise}
\end{figure}

\figref{fig:num_frames_per_instance_count} further shows the distribution of the track lengths per sequence-wise instance for each semantic class. The median track lengths range from 9.5 frames to 39 frames across classes. For some of the less frequent classes such as \emph{wheelchair} and \emph{construction vehicle}, the median track length is on the higher end, which might be due to these being generally slower moving classes. \figref{fig:instances_short_medium_long_track_length} shows an overview of the track lengths for instances stratified by class. With the non-trivial amount of short, medium, and long tracks, Panoptic nuScenes provides diversity in object track length and across a wide variety of classes. This challenges panoptic tracking approaches to be able to track objects for a relatively sustained period of time, while also being able to handle situations when an object only appears briefly.

\begin{figure}
\centering
\includegraphics[width=\linewidth]{./images/num_frames_per_instance_count.pdf}
\caption{Track length per instance for each \emph{thing} class, sorted by median track length. The triangle in a bar indicates the mean track length for the class, and the line indicates the median track length for that class.}
\label{fig:num_frames_per_instance_count}
\end{figure}

\begin{figure}
\centering
\includegraphics[width=\linewidth]{./images/instances_short_medium_long_track_length.pdf}
\caption{Distribution of the track lengths for instances stratified by class. Short tracks are tracks which persist for less than 1/3 of a scene, medium tracks are those that persist for between 1/3 and 2/3 of a scene, and long tracks are those that persist for more than 2/3 of a scene.}
\label{fig:instances_short_medium_long_track_length}
\end{figure}

\noindent\textit{Panoptic nuScenes Panoptic Segmentation and Tracking Challenges}: In Panoptic nuScenes, each LiDAR point is annotated as one of 32 semantic classes. However, for the Panoptic nuScenes panoptic segmentation and tracking challenges, we merge similar classes and remove rare or void classes, resulting in 10 \emph{thing} and 6 \emph{stuff} classes as discussed in \secref{sec:tasks_metrics}. \tableref{table:class_map} shows the class mapping from the general Panoptic nuScenes classes to the classes used in the panoptic segmentation and tracking challenges.
In addition, the rightmost column indicates the percentage of points that fall into overlapping bounding boxes for each \emph{thing} class. The panoptic labels for these points are assigned to \emph{noise}. \figref{fig:visual_ablation} presents visualizations of groundtruth annotation examples from our Panoptic nuScenes dataset for each of the three challenges. 

\begin{table}
\setlength\tabcolsep{2.0pt}
\footnotesize
\centering
\caption{Mapping from the Panoptic nuScenes classes to the challenge classes. Note that most prefixes for the former are omitted for brevity. ($^{\dagger}$) We use \emph{void} to denote classes that have been excluded from the challenges. ($^{\ddagger}$) The rightmost column shows the percentage of points within overlapping bounding boxes per class.}
\begin{tabular}{|l | C{2.0cm} | C{1.5cm}| C{1.5cm} |}
\toprule
General Panoptic Class &  Challenge Class$^{\dagger}$ &  Thing/Stuff & Overlap Percent ($\%$)$^{\ddagger}$ \\ 
\midrule
animal                                   &   void                  & thing    & 0      \\
personal mobility                        &   void                  & thing   & 0       \\
stroller                                 &   void                  & thing   & 0       \\
wheelchair                               &   void                  & thing  & 0        \\
debris                                   &   void                  & thing  & 0.12        \\
pushable                                 &   void                  & thing  & 0.7        \\
bicycle rack                             &   void                  & thing  & 0        \\ 
ambulance                                &   void                  & thing  & 0        \\ 
police                                   &   void                  & thing  & 0        \\
noise                                    &   void                  & -    & -          \\ 
other                                    &   void                  & -    & -          \\ 
ego                                      &   void                  & -    & -          \\ 
barrier                                  &   barrier               & thing  & 0.6        \\ 
bicycle                                  &   bicycle               & thing  & 0.72        \\ 
bus.bendy                                &   bus                   & thing   & 0.59       \\ 
bus.rigid                                &   bus                   & thing   & 0       \\ 
car                                      &   car                   & thing   & 0.00017       \\ 
construction                             &   construction vehicle  & thing   & 0.02       \\ 
motorcycle                               &   motorcycle            & thing   & 0.0007       \\ 
adult                                    &   pedestrian            & thing  & 0.33        \\ 
child                                    &   pedestrian            & thing  & 0.041        \\ 
construction worker                      &   pedestrian            & thing  & 0.146       \\ 
police officer                           &   pedestrian            & thing  & 0        \\ 
traffic cone                              &   traffic cone         & thing   & 0.07       \\ 
trailer                                  &   trailer               & thing   & 0.02       \\ 
truck                                    &   truck                 & thing   & 0.00249       \\ 
driveable surface                        &   driveable surface     & stuff  & -        \\ 
other                                    &   other flat            & stuff   & -       \\ 
sidewalk                                 &   sidewalk              & stuff   & -      \\ 
terrain                                  &   terrain               & stuff   & -       \\ 
manmade                                  &   manmade               & stuff   & -       \\ 
vegetation                               &   vegetation            & stuff  & -        \\
\bottomrule
\end{tabular}
\label{table:class_map}
\end{table}

\section{Additional Panoptic Segmentation Results}

In \tableref{tab:nuScenesClass}, we present a comparison of per-class panoptic segmentation results on the Panoptic nuScenes dataset. We compare the top three of our combination baselines that have published task-specific methods and the end-to-end baselines. Across all the classes, it can be seen that the independently combined baselines outperform the end-to-end methods. This is more pronounced for the \emph{thing} classes compared to the \emph{stuff} classes. Among the \emph{thing} classes, the average gap between the best-in-class result of the independently combined baselines compared to that of the end-to-end methods is 20.8 PQ, while for the \emph{stuff classes}, the average gap is 4.6 PQ. This is likely due to the role of the stronger task-specific detection methods that are used for the instance segmentation of the \emph{thing} classes.

\begin{table*}
\setlength\tabcolsep{3.7pt}
\centering
\caption{Class-wise panoptic segmentation results on the Panoptic nuScenes dataset. All scores are in [\%].}
\label{tab:nuScenesClass}
\begin{tabular}{ll|cccccccccccccccc|c}
\midrule
& Method & \begin{sideways}barrier\end{sideways} & \begin{sideways}bicycle\end{sideways} & \begin{sideways}bus\end{sideways} & \begin{sideways}car\end{sideways} & \begin{sideways}cvehicle\end{sideways} & \begin{sideways}motorcycle\end{sideways} & \begin{sideways}pedestrian\end{sideways} & \begin{sideways}traffic cone\end{sideways} & \begin{sideways}trailer\end{sideways} & \begin{sideways}truck\end{sideways} & \begin{sideways}driveable\end{sideways} & \begin{sideways}other flat\end{sideways} & \begin{sideways}sidewalk\end{sideways} & \begin{sideways}terrain\end{sideways} & \begin{sideways}man-made\end{sideways} & \begin{sideways}vegetation\end{sideways}  & PQ \\
\midrule
\multirow{3}{*}{\rotatebox[origin=c]{90}{val set}} & PanopticTrackNet~\cite{hurtado2020mopt} & 47.1 & 27.9 & 57.9 & 66.3 & 22.8 & 51.1 & 42.8 & 46.8 & 38.9 & 51.0 & 77.5 & 41.6 & 59.7 & 42.3 & 60.1 & 68.8 & 51.4  \\
& EfficientLPS~\cite{sirohi2021efficientlps} & 56.8& 37.8 & 52.4 & \textbf{75.6} & 32.1 & 65.1 & \textbf{74.9} & 73.5 & \textbf{49.9} & 49.7 & \textbf{95.2} & 43.9 & \textbf{67.5} & \textbf{52.8} & 81.8 & \textbf{82.4} & 62.0  \\
& PolarSeg-Panoptic~\cite{zhou2021panoptic} & \textbf{56.9} & \textbf{41.1} & \textbf{65.5} & 75.4 & \textbf{38.9} & \textbf{67.7} & 73.2 & \textbf{74.9} & 40.4 & \textbf{58.6} & 94.2 & \textbf{46.6} & 66.2 & 49.4 & \textbf{83.9} & 82.0 & \textbf{63.4} \\
\midrule
\multirow{6}{*}{\rotatebox[origin=c]{90}{test set}} 
& PanopticTrackNet~\cite{hurtado2020mopt} & 44.3 & 23.1 & 45.8 & 71.5 & 21.8 & 42.7 & 62.3 & 63.7 & 40.2 & 43.6 & 93.0 & 23.8 & 51.2 & 42.6 & 75.9 & 79.3 & 51.6\\
& EfficientLPS~\cite{sirohi2021efficientlps} & 57.1 & 38.1 & 53.6 & 75.8 & 31.6 & 66.0 & 75.2 & 74.3 & 50.6 & 49.4 & 95.3 & 44.1 & 68.2 & 53.3 & 82.3 & 83.4 & 62.4 \\
& PolarSeg-Panoptic~\cite{zhou2021panoptic} & 55.9 & 39.6 & 55.7 & 77.4 & 37.4 & 67.6 & 76.5 & 73.7 & 52.4 & 53.5 & 95.0 & 44.6 & 67.4 & 53.2 & 82.9 & 84.4 & 63.6 \\
& SPVNAS~\cite{tang2020searching} + CenterPoint~\cite{yin2021center} & 78.1 & 62.3 & 59.4 & 91.2 & 46.5 & 83.2 & 92.9 & 90.7 & 49.0 & 63.4 & 97.4 & 49.4 & 72.6 & 54.5 & 85.4 & 79.9 & 72.2 \\
& Cylinder3D++~\cite{zhu2021cylindrical} + CenterPoint~\cite{yin2021center} & 79.2 & 70.5 & 63.8 & \textbf{92.8} & 56.8 & 83.3 & 93.6 & 92.8 & 66.1 & 69.0 & \textbf{97.6} & \textbf{55.1} & \textbf{74.1} & \textbf{57.1} & \textbf{87.0} & \textbf{85.1} & 76.5 \\
& (AF)\textsuperscript{2}-S3Net~\cite{cheng20212} + CenterPoint~\cite{yin2021center} & \textbf{80.8} & \textbf{79.4} & \textbf{67.3} & 91.7 & \textbf{63.8} & \textbf{86.4} & \textbf{93.8} & \textbf{93.7} & \textbf{68.7} & \textbf{72.9} & 97.1 & 45.6 & 69.4 & 51.5 & 84.6 & 82.3 & \textbf{76.8} \\
\bottomrule
\end{tabular}
\end{table*}

\section{Correlation Analysis}

In this section, we extend the analysis of the combination baselines to study the relationships between (i) panoptic segmentation performance and the component semantic segmentation and detection performance, and (ii) panoptic tracking performance and the component semantic segmentation and tracking performance.

\noindent\textit{Panoptic Segmentation}: As discussed in \secref{subsec:baseline_results}, panoptic segmentation can be achieved by combining the submissions of LiDAR semantic segmentation and LiDAR detection from the nuScenes challenges. We generate 1470 of these combinations and in \figref{fig:mIoU_mAP_AMOTA_PQ_LSTQ}(a), we show an overview of the resulting panoptic segmentation performance as measured by the PQ score, for the combinations. Within each column, a perceptual change in color can be observed, implying that for the same LiDAR semantic segmentation method, the change in detection method influences the PQ. However, across each row, the change in color is insignificant, indicating that varying the LiDAR semantic segmentation method does not impact PQ as much as the LiDAR detection method.

\begin{table}
    \footnotesize
    \centering
    \caption{Correlation of LiDAR semantic segmentation methods (measured by mIoU) and tracking methods (measured by AMOTA) with various panoptic tracking metrics. The correlations are calculated from the 924 panoptic tracking baselines that we generated by combining various LiDAR semantic segmentation and tracking methods.}
    \begin{tabular}{l|c c}
    \toprule
         Metric         & AMOTA  & mIoU  \\
         \midrule
         LSTQ~\cite{aygun20214d}           & 0.55   & 0.62  \\
         PTQ~\cite{hurtado2020mopt}            & 0.23   & 0.69  \\
         PAT (Ours)           & 0.48   & 0.57  \\
         \bottomrule
    \end{tabular}
    \label{tab:correlations}
    \vspace{1cm}
\end{table}

\begin{figure*}
    \footnotesize
    \centering
    \begin{tabular}{c c}
    \includegraphics[width=0.45\linewidth]{./images/mIoU_mAP_PQ.pdf} & \includegraphics[width=0.45\linewidth]{./images/mIoU_amota_LSTQ.pdf} \\
    \\
    (a) Panoptic segmentation performance (PQ) & (b) Panoptic tracking performance (LSTQ) \\
    \end{tabular}
    \caption{Performance of panoptic segmentation and panotic tracking in relation to LiDAR semantic segmentation (mIoU) and detection (mAP) / tracking (AMOTA) performance respectively based on the combined baselines from LiDAR semantic segmentation and LiDAR detection / tracking methods.}
    \label{fig:mIoU_mAP_AMOTA_PQ_LSTQ}
\end{figure*}

\noindent\textit{Panoptic Tracking}: In \secref{subsec:new_metric_analysis}, we compare our proposed metric, PAT, with other existing metrics which has been proposed for panoptic tracking. Here, we provide additional analysis for the LSTQ metric with respect to mIoU and AMOTA metrics. \figref{fig:mIoU_mAP_AMOTA_PQ_LSTQ}(b) gives a qualitative overview of how LSTQ varies with different panoptic tracking baselines which we generate by combining LiDAR semantic segmentation and tracking methods. As per \secref{subsec:baseline_results}, we used mIoU and AMOTA as a performance measure for the LiDAR semantic segmentation methods and the tracking methods respectively. From the 924 independently combined panoptic tracking baselines, we can see that there is generally a perceptual change in color across each row and column. This implies that LSTQ takes into account both the LiDAR semantic segmentation performance as well as the tracking performance. In \tableref{tab:correlations}, we show more quantitatively how various panoptic tracking metrics consider LiDAR semantic segmentation and tracking. PTQ demonstrates more bias towards LiDAR semantic segmentation as observed from the significantly stronger correlation between mIoU and PTQ in contrast to that between AMOTA and PTQ. On the other hand, LSTQ and PAT are more balanced metrics, with a smaller disparity in the respective correlations.

%\footnotesize
%\bibliographystyleNew{IEEEtran}
%\bibliographyNew{references_appendix.bib}
